# Supplementary material for: Extracting Quantum Many-Body Scarred Eigenstates with Matrix Product States
Source: arXiv:2211.05140 source file (2023-07-12)

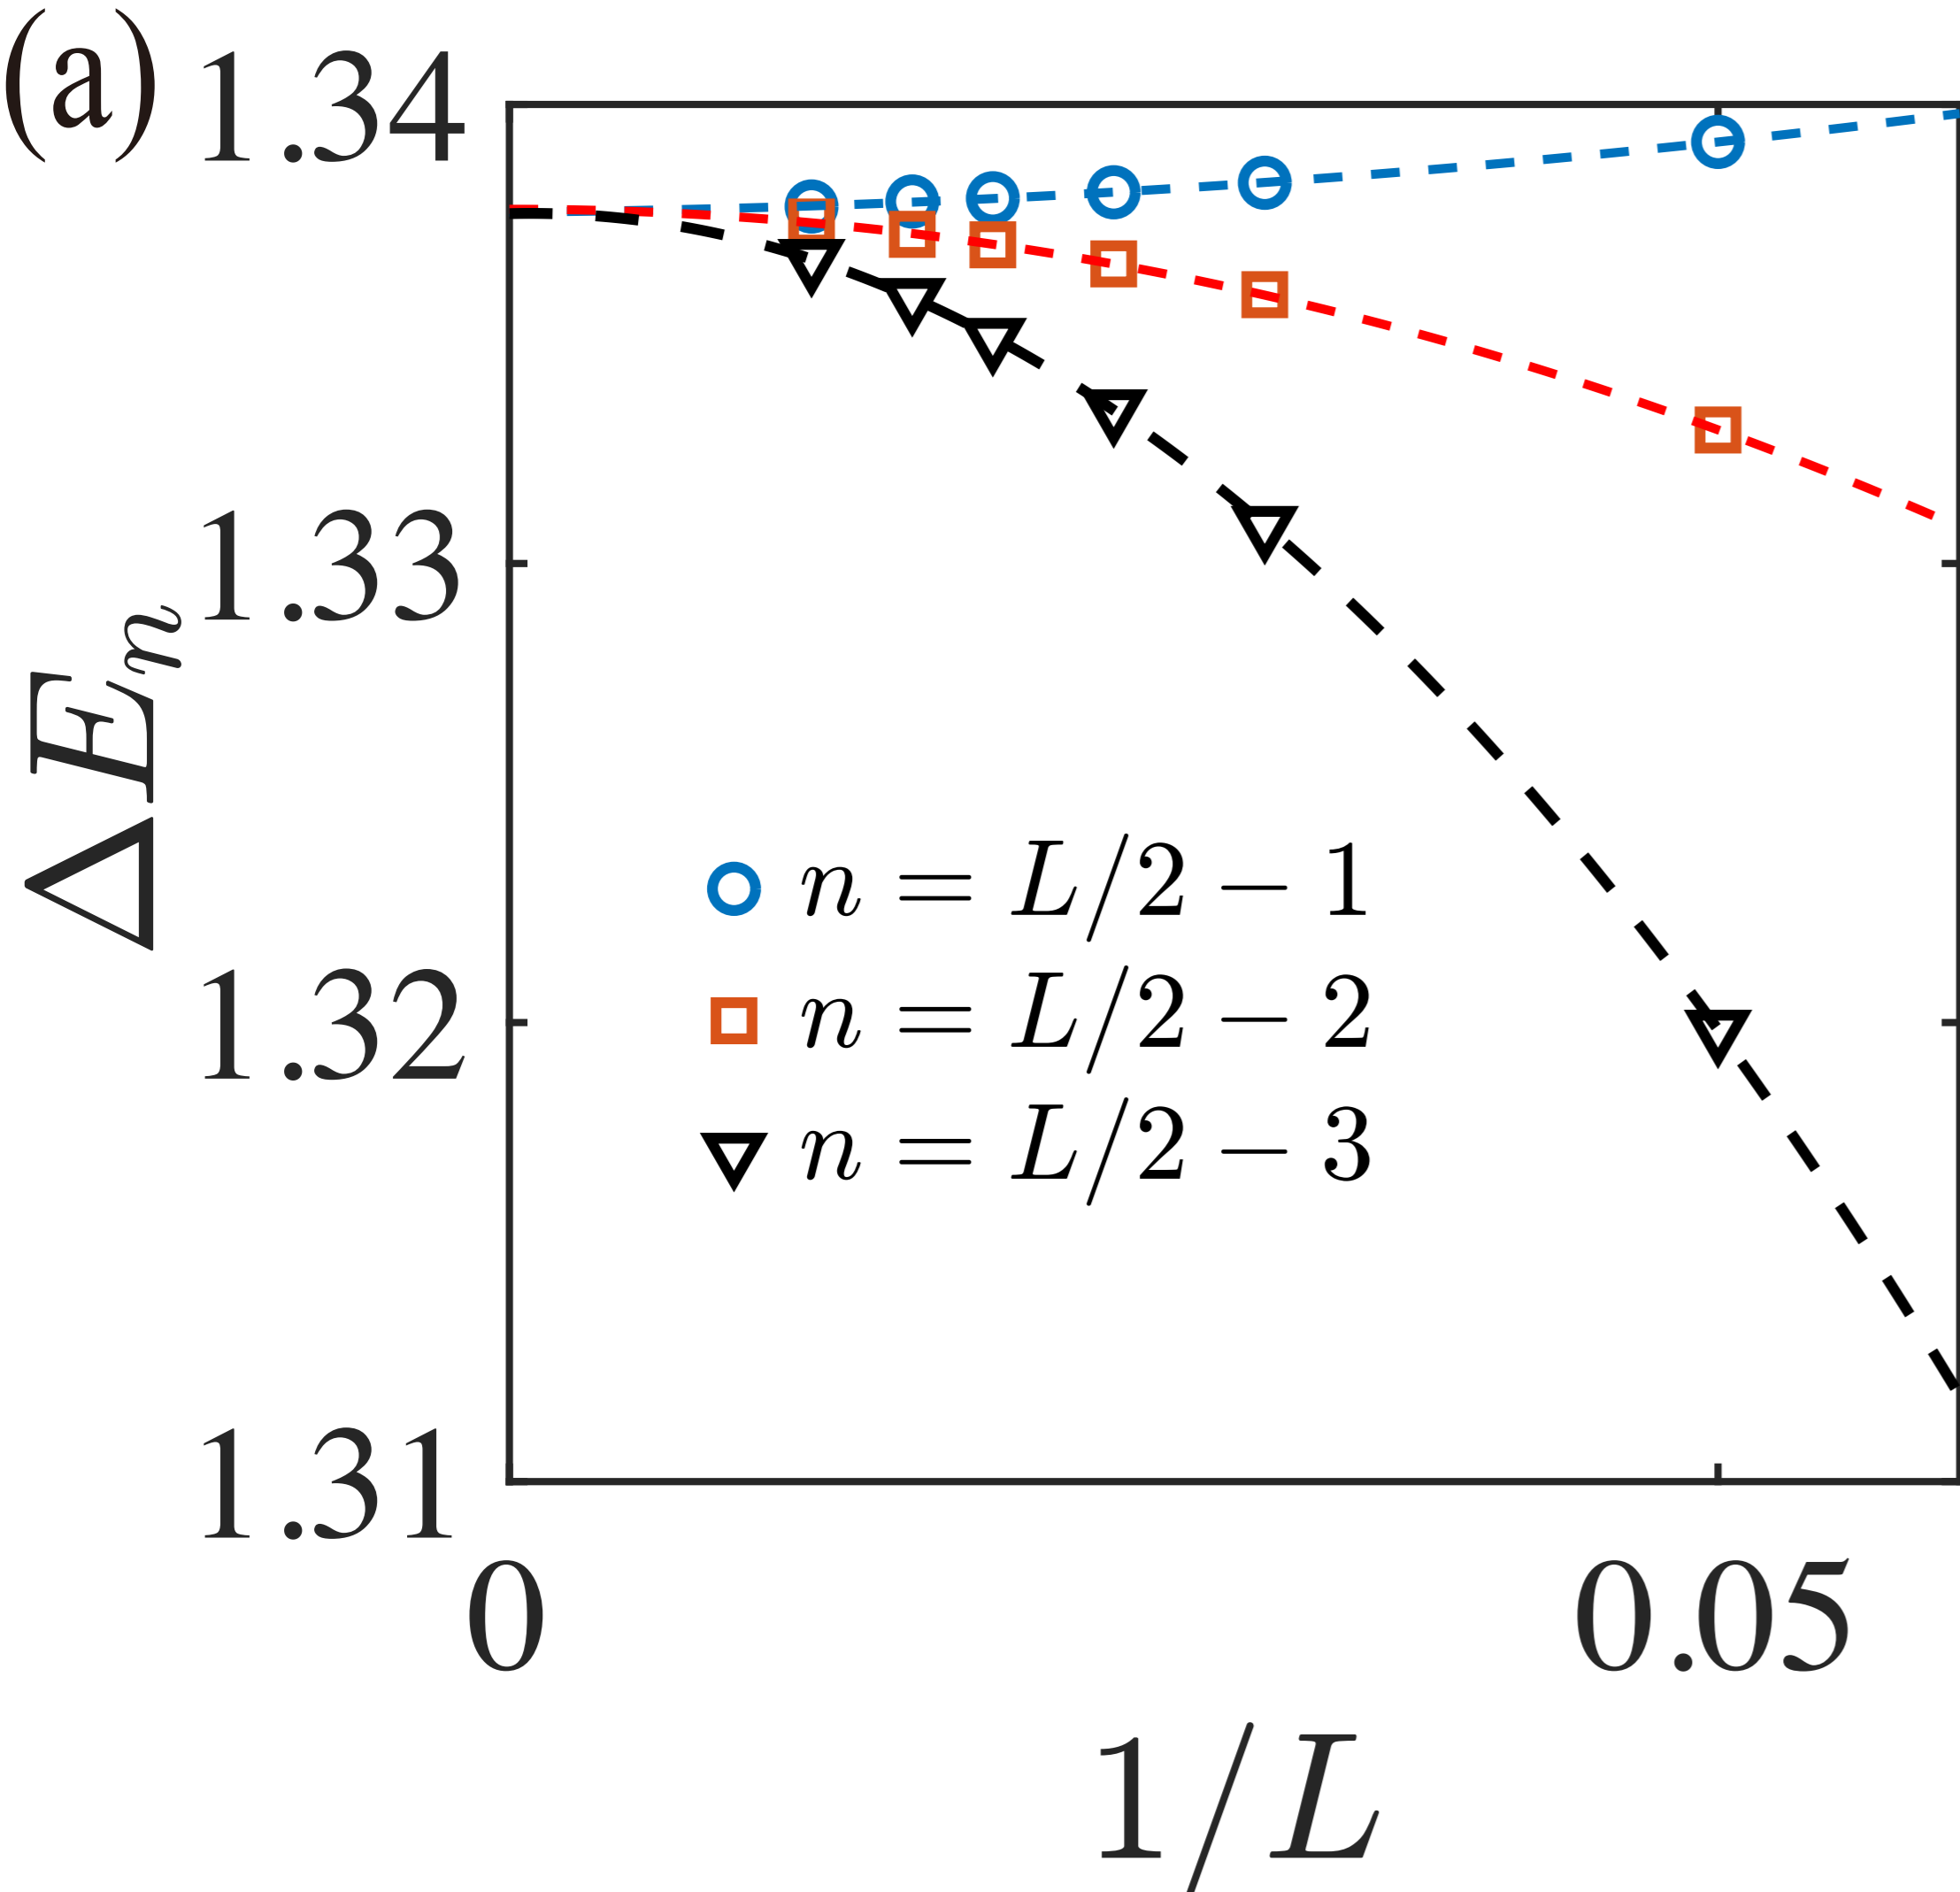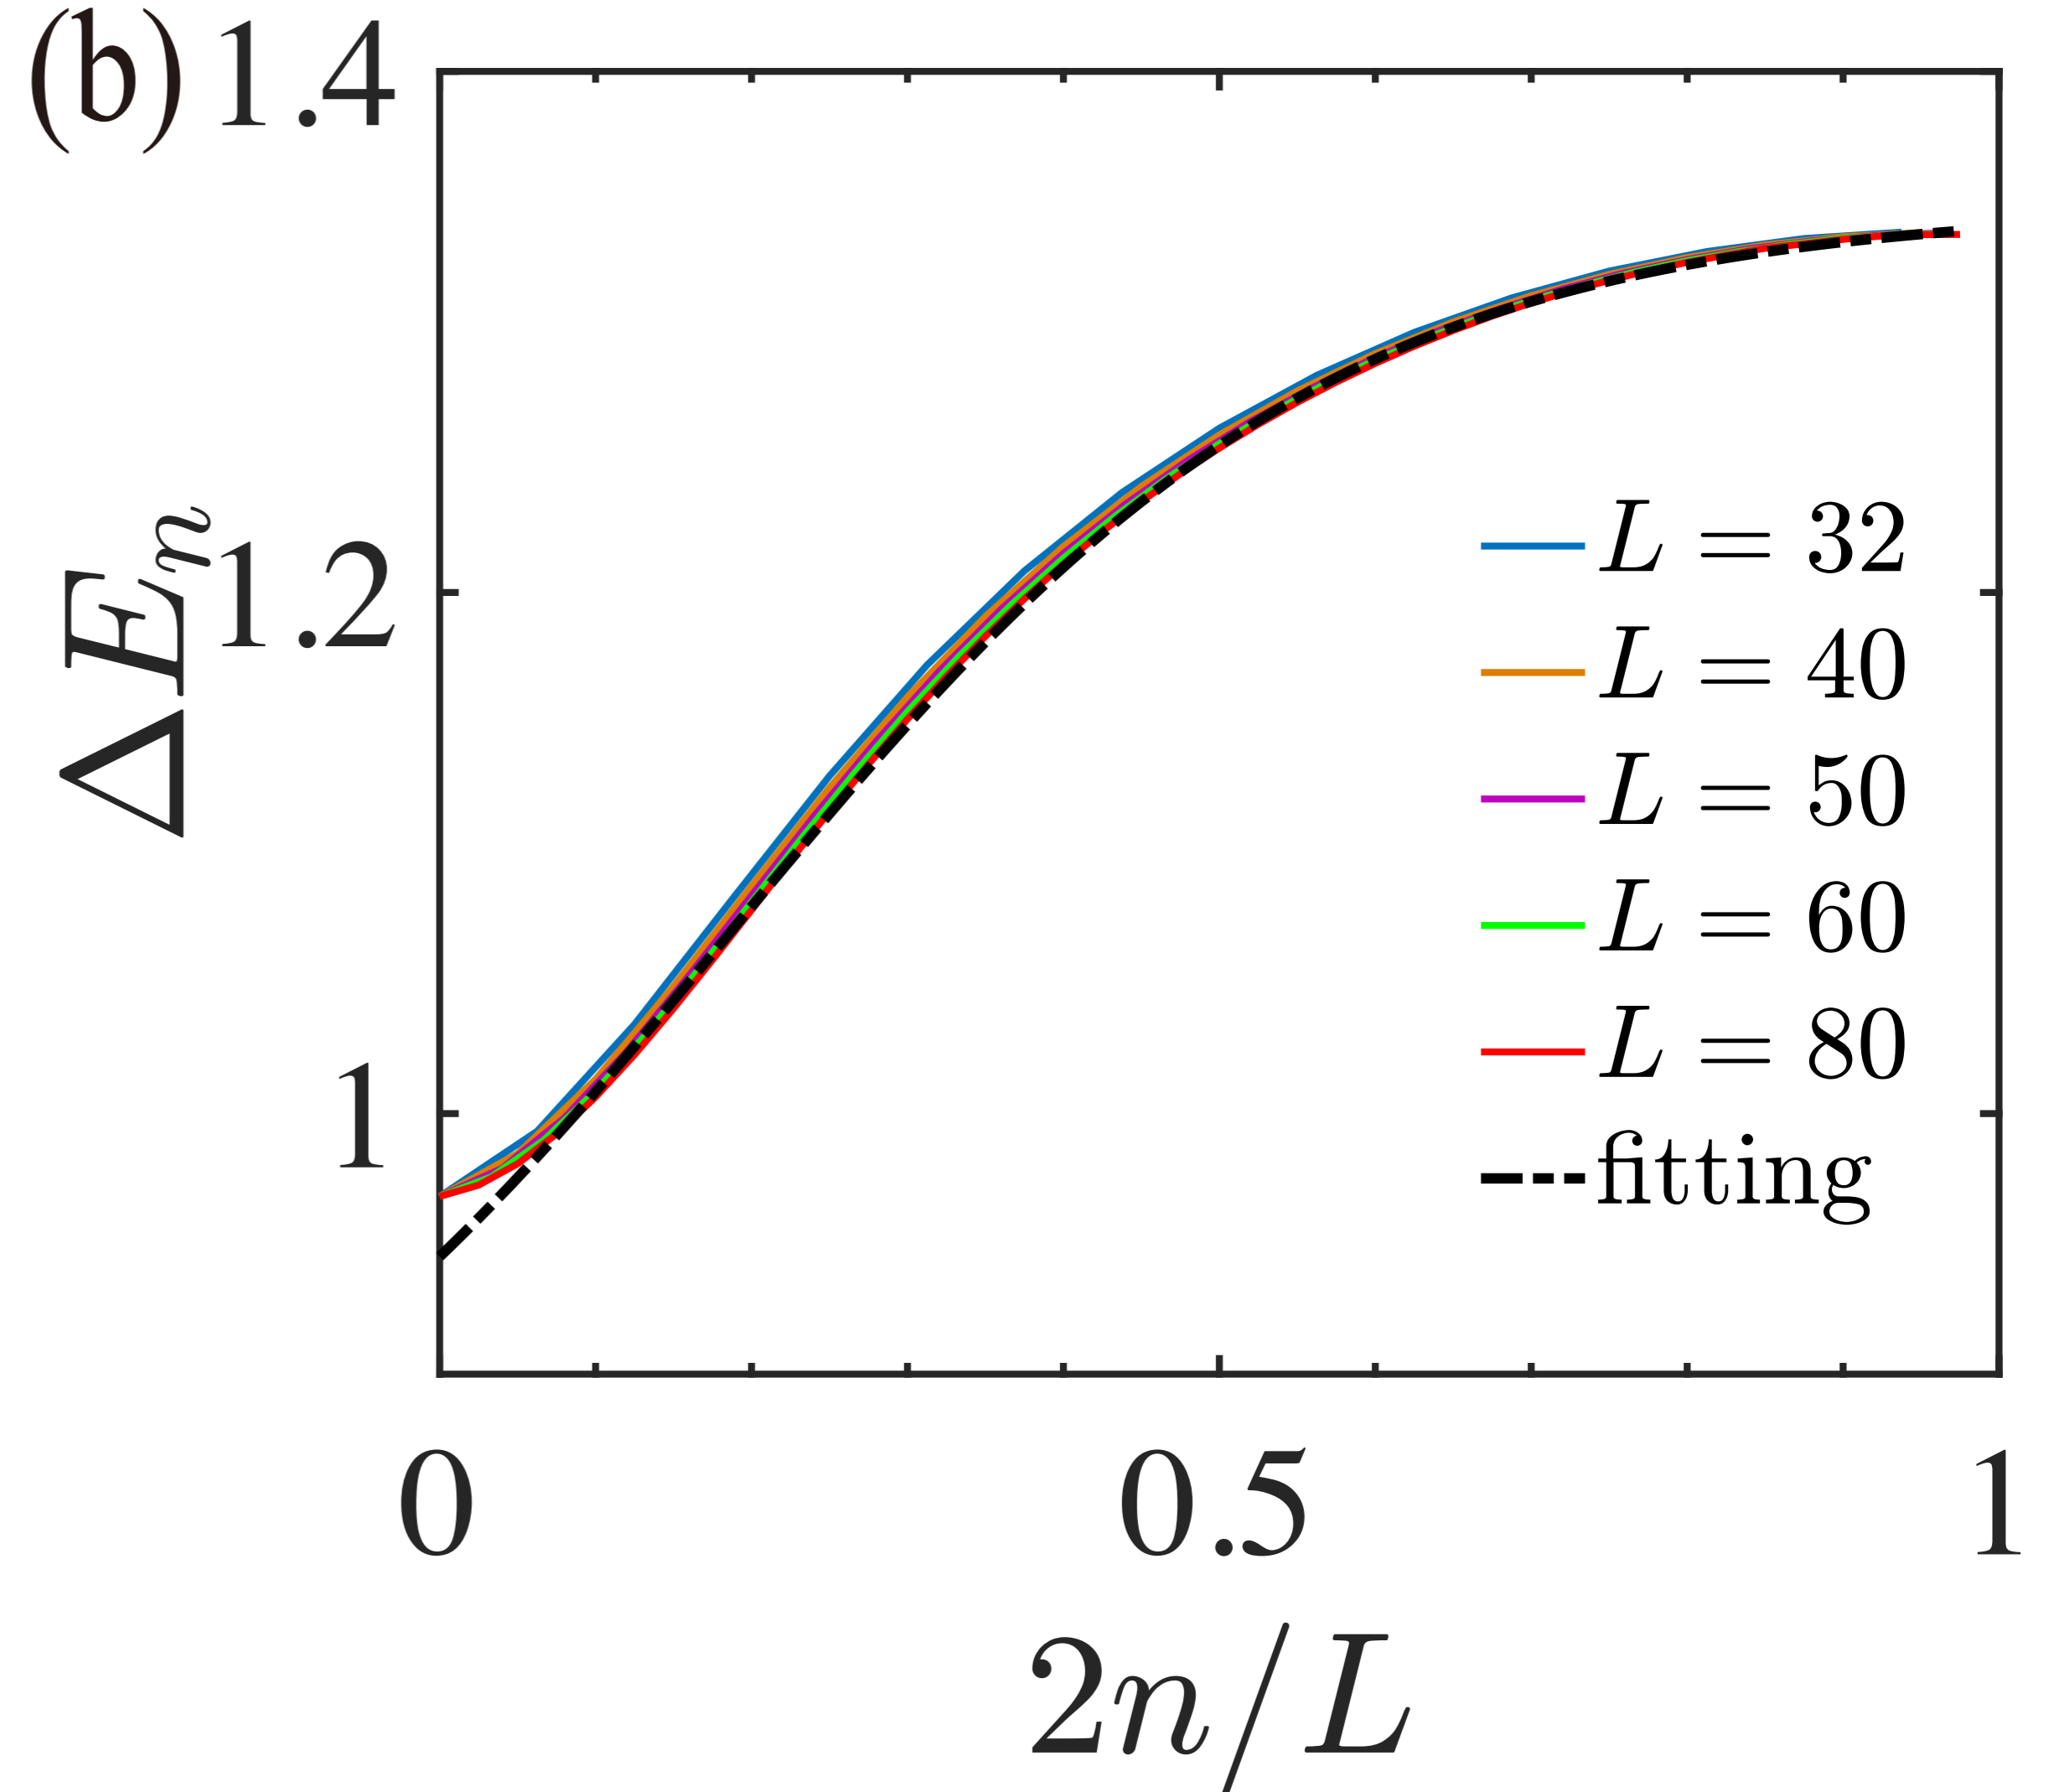

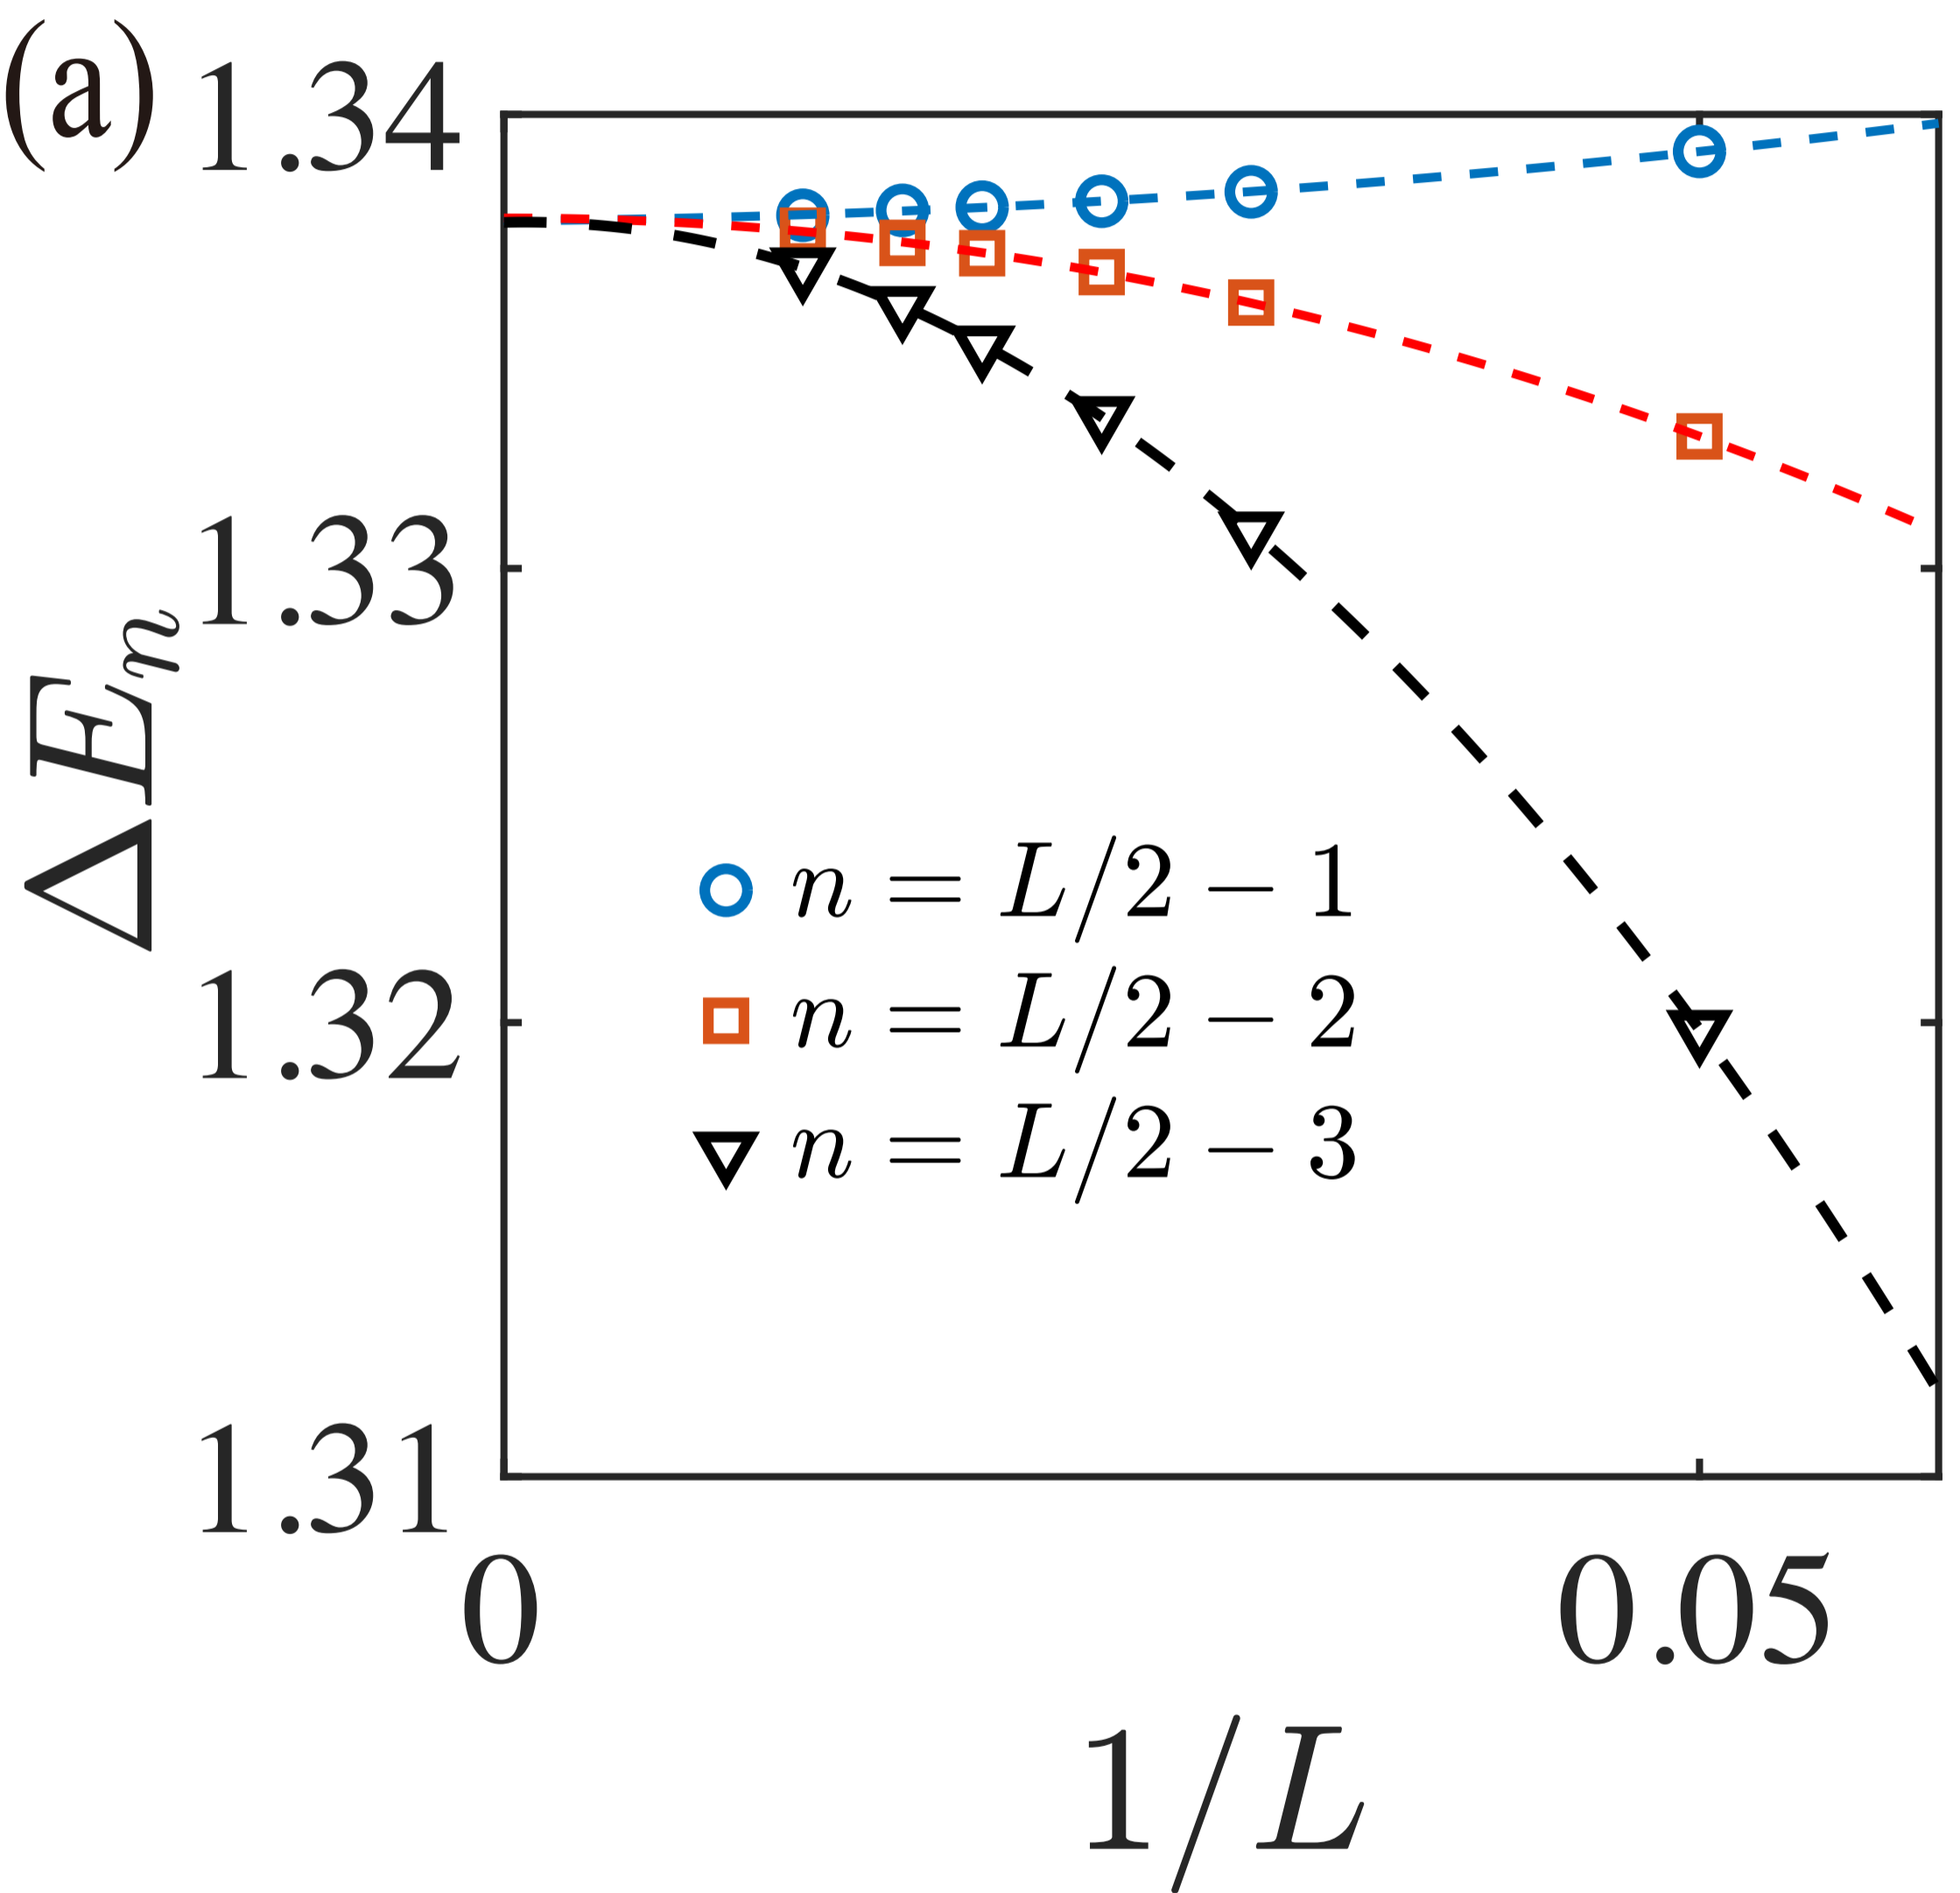

Supplement: Supplementary file 1 [file fit_SM.pdf]
